# Supplementary material for: Simudo: a device model for intermediate band materials
Source: arXiv:1905.11303 source file (2019-10-21)
Supplement: Supplementary file 1 [file Simudo_Supplementary_Info.pdf]

Supplementary Information
Simudo: a device model for intermediate band materials
Eduard C. Dumitrescu, Matthew M. Wilkins, and Jacob J. Krich

## equilibrium.py

```
"""
Set up a simple device model and solve for thermal equilibrium.
"""

import logging
from simudo.fem import setup_dolfin_parameters
from simudo.mesh import (CellRegions, ConstructionHelperLayeredStructure, FacetRegions)
from simudo.physics import (ProblemData, SimpleSiliconMaterial)
from simudo.util import make_unit_registry

U = make_unit_registry(("mesh_unit = 1 micrometer",))
setup_dolfin_parameters()
doping = 1e18 * U('cm^-3') # doping level for both sides

#####
# Define geometry of layers, including names for easy referencing
#####
mesh_points = 400 ; L = 0.2 # device length in um
layers = [dict(name='emitter', material='Si', thickness=L/2),
          dict(name='base'   , material='Si', thickness=L/2)]

# For non-uniform meshing, define regions to receive extra mesh points
# "+/-layer" indicates relative to right/left endpoint of layer
overmesh_regions = [
  dict(x0=('-emitter', -L/20), x1=('-emitter', +L/20), edge_length=L*1e-4),
  dict(x0=('+base'   , -L/20), x1=('+base'   , +L/20), edge_length=L*1e-4)]

# Helper for constructing 1D models from a list of layers
ls = ConstructionHelperLayeredStructure()
ls.params = dict(edge_length=L/mesh_points, # default edge_length
  layers=layers, simple_overmesh_regions=overmesh_regions, mesh_unit=U.mesh_unit)
ls.run()
mesh_data = ls.mesh_data

# topology: define names for certain external facets of the domain
R, F = CellRegions(), FacetRegions()
F.exterior = (R.domain).boundary(R.exterior)
F.left_contact  = (R.exterior_left).boundary(R.domain)
F.right_contact =        (R.domain).boundary(R.exterior_right)
F.contacts = F.left_contact | F.right_contact
F.nonconductive = F.exterior – F.left_contact.flip() - F.right_contact

#####
# Define PDD problem, including bands, BC's, and recombination
#####
def create_problemdata(goal, phi_charge_neutrality=None):
  root = ProblemData(goal=goal, mesh_data=mesh_data, unit_registry=U)
  pdd = root.pdd
  pdd.easy_add_band(name='CB', band_type=None)
  pdd.easy_add_band(name='VB', band_type=None)
  pdd.spatial.add_rule('temperature', R.domain, U('300 K'))
```

```
  # p-type doping
  pdd.spatial.add_rule('poisson/static_rho', R.emitter, -doping *
U('elementary_charge'))
  # n-type doping
  pdd.spatial.add_rule('poisson/static_rho', R.base   , +doping *
U('elementary_charge'))

  pdd.spatial.add_rule('SRH/CB/tau'      , R.domain, U('1e-9 s'))
  pdd.spatial.add_rule('SRH/VB/tau'      , R.domain, U('1e-6 s'))
  pdd.spatial.add_rule('SRH/energy_level', R.domain, U('0.553 eV'))

  # Assign silicon material library properties to all regions containing silicon
  SimpleSiliconMaterial(problem_data=root).register()

  # For Step 2, assign phi to charge neutrality value at contacts, E-field to 0 at
nonconductive boundaries.
  if goal == 'thermal equilibrium':
    pdd.spatial.add_BC('poisson/phi', F.contacts     , phi_charge_neutrality)
    pdd.spatial.add_BC('poisson/E'  , F.nonconductive, U('V/m') *
pdd.mesh_util.zerovec)
  return root

#####
# Run pre-solver
#####
p0 = create_problemdata(goal='local charge neutrality')
p0.pdd.easy_auto_pre_solve()                                          # Step 1
p1 = create_problemdata(goal='thermal equilibrium',
                        phi_charge_neutrality=p0.pdd.poisson.phi)
p1.pdd.easy_auto_pre_solve()                                          # Step 2
```

```
"""
Generate output for comparison with 'A. Martí, L.  Cuadra and A. Luque, "Quasi-drift
diffusion model for the quantum dot intermediate band solar cell", IEEE Trans. Elec.
Dev., vol 49 (9), pp. 1632-1639 (2002).'
"""


from simudo.physics import (
    Material,
    ProblemData,
    PoissonDriftDiffusion,
    SRHRecombination, NonRadiativeTrap,
    NonOverlappingTopHatBeerLambert,
    NonOverlappingTopHatBeerLambertIB)

from simudo.mesh import (
    ConstructionHelperLayeredStructure,
    Interval, CInterval, CellRegions, FacetRegions)

from simudo.fem import setup_dolfin_parameters

from simudo.util import (
    make_unit_registry, DictAttrProxy,
    TypicalLoggingSetup)

from simudo.io import h5yaml

from functools import partial
from cached_property import cached_property
import pandas as pd
import numpy as np
import os
from os import path as osp
from argh import ArghParser, arg
import itertools
from atomicwrites import atomic_write

import dolfin
import logging

def dirname(path):
    return os.path.join(os.path.dirname(path + 'x'), 'x').rstrip('x')

class Semiconductor(Material):
    name = 'semiconductor'
    def get_dict(self):
        d = super().get_dict()
        U = self.unit_registry

        d.update({
            # band parameters
            'CB/energy_level': U('1.67 eV'),
            'IB/energy_level': U('1.10 eV'),
            'VB/energy_level': U('0 eV'),

            'IB/degeneracy': 1,

            'CB/effective_density_of_states': U('5e18 1/cm^3'),
            'VB/effective_density_of_states': U('5e18 1/cm^3'),
            'IB/number_of_states': U('1e4 cm^-3'),
```

```python
            # electrical properties
            'CB/mobility': U('2000 cm^2/V/s'),
            'VB/mobility': U('2000 cm^2/V/s'),
            'IB/mobility': U('62 cm^2/V/s'),

            # meaningless
            'opt_ci/sigma_opt': U('1e-17 cm^2'),
            'opt_iv/sigma_opt': U('1e-17 cm^2'),

            'opt_cv/alpha': U('1e4 cm^-1'),

            # 'nr_top/v_th': U('2.042e7 cm/s'),
            # 'nr_bottom/v_th': U('1.562e7 cm/s'),
            # 'nr_top/sigma_th': U('1e-18 cm^2'),
            # 'nr_bottom/sigma_th': U('1e-18 cm^2'),

            # poisson
            'poisson/permittivity': U('13 vacuum_permittivity'),
        })
        return d

class IBSemiconductor(Semiconductor):
    name = 'IB'

    def get_dict(self):
        d = super().get_dict()
        U = self.unit_registry

        d.update({
            # these cross sections give alpha=1e4/cm at half-filled IB
            # `1e4 / (1e17/2.)`
            'opt_ci/sigma_opt': U('2e-13 cm^2'),
            'opt_iv/sigma_opt': U('2e-13 cm^2'),

            'IB/number_of_states': U('1e17 cm^-3')
        })

        return d

class PFrontSurfaceField(Semiconductor):
    name = 'pfsf'

    def get_dict(self):
        d = super().get_dict()
        U = self.unit_registry

        d['opt_cv/alpha'] = U('0 cm^-1')

        return d

def topology_standard_contacts(cell_regions, facet_regions):
    R, F = cell_regions, facet_regions

    F.left_contact  = lc = R.exterior_left.boundary(R.domain        )
    F.right_contact = rc = R.domain       .boundary(R.exterior_right)

    F.exterior = R.domain.boundary(R.exterior)
    F.contacts = lc | rc
    F.nonconductive = F.exterior - F.contacts.both()


def submitfile_to_title(submitfile_tree):
    p = submitfile_tree['parameters']
```

```python
    title = ("marti02 X={concentration_factor} mu={IB_mobility} "
             "s_ci={IB_sigma_ci} s_iv={IB_sigma_iv}".format(**p))

    return title

def generate(output_prefix='out/'):

    output_prefix = output_prefix.rstrip('/') + '/'

    def write(data, filename):
        os.makedirs(dirname(filename), exist_ok=True)
        h5yaml.dump(data, filename)

    concentration_factors = [
        # '0',
        '1e3',
    ]
    mobilities = [
        '0.001',
        '0.01',
        '0.1',
        '1',
        '3',
        '10',
        '30',
        '100',
        '300',
    ]
    IB_sigma_cis = ['2e-13', '1e-12']

    for X, mu, s_ci in itertools.product(
            concentration_factors, mobilities,
            IB_sigma_cis):

        tree = dict(concentration_factor=X,
                    IB_mobility=mu,
                    IB_thickness='1.3',
                    IB_sigma_ci=s_ci,
                    IB_sigma_iv='2e-13',
                    title=None)

        submitfile_tree = dict(parameters=tree)

        title = submitfile_to_title(submitfile_tree)
        submitfile_tree['parameters']['title'] = title

        outfile = output_prefix + title + '/submit.yaml'

        if os.path.exists(outfile):
            continue

        write(submitfile_tree, outfile)

@arg('submitfiles', nargs='*')
def fixup_titles(submitfiles):
    for submitfile in submitfiles:
        t = h5yaml.load(submitfile)
        p = t['parameters']
        p.setdefault('IB_sigma_ci', '2e-13')
        p.setdefault('IB_sigma_iv', '2e-13')

        p['title'] = title = submitfile_to_title(t)

        with atomic_write(submitfile, overwrite=True) as f:
```

```
        h5yaml.dump(t, f)

    olddir = osp.dirname(submitfile)
    newdir = osp.join(osp.dirname(olddir), title)
    os.rename(olddir, newdir)

def run(submitfile):
    U = make_unit_registry(("mesh_unit = 1 micrometer",))

    PREFIX = dirname(submitfile)
    submitfile_data = h5yaml.load(submitfile)
    P = submitfile_data['parameters']

    TypicalLoggingSetup(filename_prefix=PREFIX).setup()

    setup_dolfin_parameters()

    layers = [
        dict(name='pfsf', material='pfsf'         ,
             thickness=0.05),
        dict(name='p'   , material='semiconductor',
             thickness=1.0),
        dict(name='I'   , material='IB'           ,
             thickness=float(P['IB_thickness'])),
        dict(name='n'   , material='semiconductor',
             thickness=1.0)]

    # -layer means relative to left endpoint of layer
    # +layer means relative to right endpoint of layer
    simple_overmesh_regions = [
        dict(x0=('-pfsf', -0.15), x1=('-pfsf', +0.15), edge_length=0.001 ),
        dict(x0=('+p'   , -0.05), x1=('+p'   , +0.05), edge_length=0.0005),
        dict(x0=('+I'   , -0.05), x1=('+I'   , +0.05), edge_length=0.0005),
        dict(x0=('+n'   , -0.1 ), x1=('+n'   , +0.1 ), edge_length=0.001 ),
    ]

    ls = ConstructionHelperLayeredStructure()
    ls.params = dict(edge_length=0.01, # default edge length
                     layers=layers,
                     simple_overmesh_regions=simple_overmesh_regions,
                     mesh_unit=U.um)
    ls.run()
    mesh_data = ls.mesh_data

    if True:
        Xs_df = pd.DataFrame({
            'X': list(sorted(set(mesh_data.mesh.coordinates()[:,0])))})
        Xs_df.to_csv(PREFIX+"mesh_Xs.csv")

    if False:
        print("exiting early")
        return

    logging.getLogger('main').info("NUM_MESH_POINTS: {}".format(
        len(ls.interval_1d_tag.coordinates['coordinates'])))

    ## topology
    R = CellRegions()
    F = FacetRegions()

    topology_standard_contacts(R, F)

    R.cell = R.p | R.n | R.I | R.pfsf
```

```python
    F.p_contact   = F.left_contact
    F.pI_junction = R.p.boundary(R.I)
    F.In_junction = R.I.boundary(R.n)
    F.n_contact   = F.right_contact

    F.IB_junctions = F.pI_junction | F.In_junction
    ## end topology


    def create_problemdata(
            goal='full', V_ext=None, phi_cn=None):
        """
goal in {'full', 'local neutrality', 'thermal equilibrium'}
"""
        root = ProblemData(
            goal=goal,
            mesh_data=mesh_data,
            unit_registry=U)
        pdd = root.pdd

        CB = pdd.easy_add_band('CB')
        IB = pdd.easy_add_band('IB')
        VB = pdd.easy_add_band('VB')

        # material to region mapping
        spatial = pdd.spatial

        spatial.add_value_rule(
            R.domain, 'temperature', U('300 K'))

        spatial.add_value_rule(
            R.p, 'poisson/static_rho', U('-1e17 elementary_charge/cm^3'))
        spatial.add_value_rule(
            R.n, 'poisson/static_rho', U('+1e17 elementary_charge/cm^3'))
        spatial.add_value_rule(
            R.pfsf, 'poisson/static_rho', U('-1e19 elementary_charge/cm^3'))
        spatial.add_value_rule(
            R.I, 'poisson/static_rho', U('+0.5e17 elementary_charge/cm^3'))

        ib_material = IBSemiconductor(problem_data=root)
        ib_material.dict['IB/mobility'] = (
            float(P['IB_mobility'])*U('cm^2/V/s'))
        for k in ['ci', 'iv']:
            ib_material.dict['opt_{}/sigma_opt'.format(k)] = (
                float(P['IB_sigma_{}'.format(k)]) * U('cm^2'))

        PFrontSurfaceField(problem_data=root).register()
        semiconductor_material = Semiconductor(problem_data=root)

        ib_material.register()
        semiconductor_material.register()


        mu = pdd.mesh_util

        zeroE = F.exterior

        if goal == 'full':
            optical = root.optical
            ospatial = optical.spatial

            def _ediff(lower, upper):
                d = semiconductor_material.dict
```

```python
    return ((d[upper+'/energy_level'] -
             d[lower+'/energy_level']) +
            U('1e-10 eV'))

optical.easy_add_field(
    'forward_ci', photon_energy=_ediff('IB', 'CB'),
    direction=(1.0, 0.0))

optical.easy_add_field(
    'forward_iv', photon_energy=_ediff('VB', 'IB'),
    direction=(1.0, 0.0))

optical.easy_add_field(
    'forward_cv', photon_energy=_ediff('VB', 'CB'),
    direction=(1.0, 0.0))

from simudo.util import Blackbody
bb = Blackbody(temperature=6000*U.K)

ofield_E_keys = ('forward_cv', 'forward_ci', 'forward_iv')
for name, (lower, upper) in bb.non_overlapping_energy_ranges(
        {name: optical.fields[name].photon_energy
        for name in ofield_E_keys}).items():
    flux = bb.photon_flux_integral_on_earth(
        lower, upper) * float(P['concentration_factor'])
    flux = flux.to('1/cm^2/s')
    ospatial.add_BC(name+'/Phi', F.left_contact, flux)
    logging.getLogger('main').info(
        "Input photon flux for field {!r}: {}"
        .format(name, flux))

pdd.easy_add_electro_optical_process(
    NonOverlappingTopHatBeerLambertIB,
    name='opt_ci',
    dst_band=CB, src_band=IB, trap_band=IB)

pdd.easy_add_electro_optical_process(
    NonOverlappingTopHatBeerLambertIB,
    name='opt_iv',
    dst_band=IB, src_band=VB, trap_band=IB)

pdd.easy_add_electro_optical_process(
    NonOverlappingTopHatBeerLambert,
    name='opt_cv',
    dst_band=CB, src_band=VB)

# pdd.easy_add_electro_optical_process(
#     SRHRecombination, dst_band=CB, src_band=VB, name='SRH')

# NonRadiativeTrap.easy_add_two_traps_to_pdd( pdd, 'nr',
#                                              CB, VB, IB)

spatial.add_BC('CB/j', F.nonconductive,
               U('A/cm^2') * mu.zerovec)
spatial.add_BC('VB/j', F.nonconductive,
               U('A/cm^2') * mu.zerovec)
spatial.add_BC('IB/j', F.exterior,
               U('A/cm^2') * mu.zerovec)

# majority contact
spatial.add_BC('VB/u', F.p_contact,
               VB.thermal_equilibrium_u)
spatial.add_BC('CB/u', F.n_contact,
               CB.thermal_equilibrium_u)
```

```python
        # minority contact
        spatial.add_BC('VB/u', F.n_contact,
                       VB.thermal_equilibrium_u)
        spatial.add_BC('CB/u', F.p_contact,
                       CB.thermal_equilibrium_u)

        phi0 = pdd.poisson.thermal_equilibrium_phi
        spatial.add_BC('poisson/phi', F.p_contact,
                       phi0 + V_ext)
        spatial.add_BC('poisson/phi', F.n_contact,
                       phi0)

        zeroE -= (F.p_contact | F.n_contact).both()

    elif goal == 'thermal equilibrium':
        # to match old method, use local charge neutrality phi as
        # the phi boundary condition for Poisson-only thermal
        # equilibrium
        spatial.add_BC('poisson/phi', F.p_contact | F.n_contact,
                       phi_cn)
        zeroE -= (F.p_contact | F.n_contact).both()

    spatial.add_BC('poisson/E', zeroE,
                   U('V/m') * mu.zerovec)

    return root

problem = create_problemdata(goal='local charge neutrality')

problem.pdd.easy_auto_pre_solve()

problem0 = problem
problem = create_problemdata(goal='thermal equilibrium',
                             phi_cn=problem0.pdd.poisson.phi)
problem.pdd.initialize_from(problem0.pdd)

problem.pdd.easy_auto_pre_solve()

V_ext = U.V * dolfin.Constant(0.0)
problem0 = problem
problem = create_problemdata(goal='full', V_ext=V_ext)
problem.pdd.initialize_from(problem0.pdd)

from simudo.physics import (
    VoltageStepper, OpticalIntensityAdaptiveStepper)
from simudo.io.output_writer import (
    OutputWriter, MetaExtractorBandInfo,
    MetaExtractorIntegrals)

meta_extractors = (
    MetaExtractorBandInfo,
    partial(MetaExtractorIntegrals,
            facets=F[{'p_contact', 'n_contact'}],
            cells=R[{'pfsf', 'p', 'n', 'I'}]))

optics = float(P['concentration_factor']) != 0

if optics:
    optical_rampup_start_logparam = 20
    stepper = OpticalIntensityAdaptiveStepper(
        solution=problem,
        # parameter_target_values=[1e-10, 0.1, 1.0],
        parameter_target_values=[0]+[
```

```
                10**-n for n in
                range(0, optical_rampup_start_logparam+1, 4)[::-1]],
            step_size=10**-optical_rampup_start_logparam,
            # step_size=0.5,
            output_writer=OutputWriter(
                filename_prefix=PREFIX+"I", plot_1d=True, plot_iv=False,
                meta_extractors=meta_extractors),
            selfconsistent_optics=True)

        stepper.do_loop()

    V_exts = list(np.linspace(0, 1.5, 75+1))
    V_exts.extend(np.linspace(1.15, 1.30, 75+1))
    V_exts = list(set(V_exts))
    V_exts.sort()

    stepper = VoltageStepper(
        solution=problem, constants=[V_ext],

        # parameter_target_values=[1.0],
        # step_size=0.5,

        parameter_target_values=V_exts,

        # parameter_target_values=np.arange(0, 12)*0.1,

        parameter_unit=U.V,
        output_writer=OutputWriter(
            filename_prefix=PREFIX+"a", plot_1d=True, plot_iv=False,
            meta_extractors=meta_extractors),
        selfconsistent_optics=optics)

    stepper.do_loop()

    return locals()

parser = ArghParser()
parser.add_commands([generate, run, fixup_titles])

if __name__ == '__main__':
    parser.dispatch()
```
